# Supplementary material for: MetaFood3D: 3D Food Dataset with Nutrition Values
Source: arXiv:2409.01966 source file (2024-12-07)
Supplement: Supplementary file 1 [file supplementary.tex]

\clearpage
\setcounter{page}{1}
\maketitlesupplementary

\definecolor{mintblue}{RGB}{173,216,230}
\definecolor{skyblue}{RGB}{78,182,255}
\definecolor{lightred}{RGB}{253,226,228}
\definecolor{lightpurple}{RGB}{223,230,253}

\section*{Overview}
This section provides comprehensive information on our MetaFood3D datasets and detailed implementation specifications for our experiments. Due to the large file size of the complete dataset, we have included only the 3D point clouds of all 743 food items and corresponding nutrition values in the supplementary zip file. The point clouds provided are randomly sampled from the mesh with 1024 points and 4096 points. The full dataset, including all annotations, will be made publicly available.

\section{Dataset Information}

\textbf{Data distribution:} In this supplementary material, we present a comprehensive distribution figure (Figure \ref{fig:class_dist_suppl}) that includes the names of all categories.

\textbf{Intended uses:} In experiments section of the main paper, we showcase the intended uses of our dataset. These include 3D food perception, novel view synthesis, 3D mesh reconstruction, 3D food object generation, synthetic food intake scene image and data generation, 3D food object texture augmentation, and food portion estimation. The dataset is created to facilitate tasks and downstream applications in both the dietary assessment domain and the 3D vision domain.

\textbf{Example nutrition values and video captures}: Due to space constraints in the main paper, we provide an example here showcasing the nutritional values associated with our dataset in Table \ref{tab:nutri_tab_suppl}.
Additionally, we present examples of our video captures and the provided object masks, as illustrated in Figure \ref{fig:video_capture_examples}. 

% \begin{figure}[h]
%     \centering
%     \includegraphics[width=\linewidth]{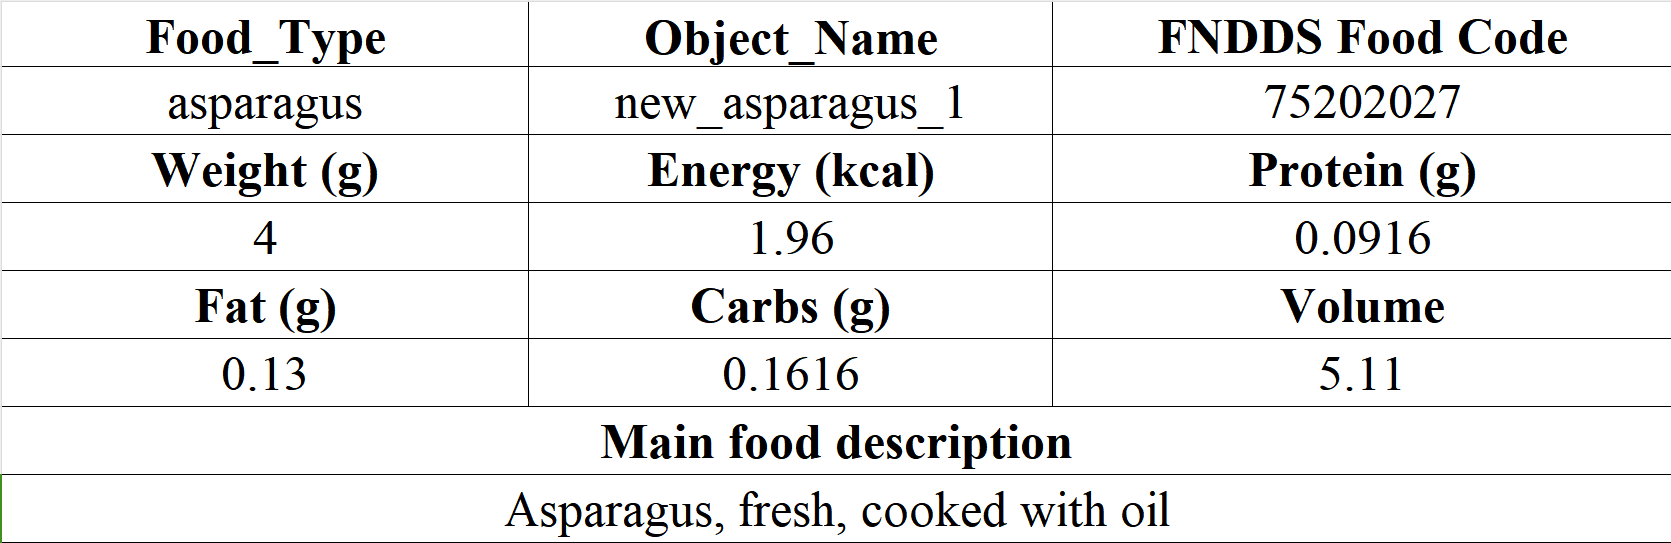}
%     \caption{Nutritional information of a food sample from MetaFood3D}
%     \label{fig:nutri_tab_suppl}
% \end{figure}

\begin{table}[h!]
    \centering
    \setlength{\arrayrulewidth}{0.5mm}
    
    \resizebox{\columnwidth}{!}{%
    \begin{tabular}{|>{\centering\arraybackslash}m{4cm}|>{\centering\arraybackslash}m{4cm}|>{\centering\arraybackslash}m{4cm}|}
        \hline
        \textbf{Food Type} & \textbf{Object Name} & \textbf{FNDDS Food Code} \\ \hline
        asparagus & new\_asparagus\_1 & 75202027 \\ \hline
        \textbf{Weight (g)} & \textbf{Energy (kcal)} & \textbf{Protein (g)} \\ \hline
        4 & 1.96 & 0.0916 \\ \hline
        \textbf{Fat (g)} & \textbf{Carbs (g)} & \textbf{Volume} \\ \hline
        0.13 & 0.1616 & 5.11 \\ \hline
        \multicolumn{3}{|c|}{\textbf{Main Food Description}} \\ \hline
        \multicolumn{3}{|c|}{Asparagus, fresh, cooked with oil} \\ \hline
    \end{tabular}
    }
    \caption{Nutritional information of a food sample from MetaFood3D}
    \label{tab:nutri_tab_suppl}
\end{table}

\begin{figure*}
    \centering
    \includegraphics[width=\linewidth]{images/food_dist_updated_suppl.png}
    \caption{MetaFood3D Overview: Complete Distribution of Food Samples by Class.}
    \label{fig:class_dist_suppl}
\end{figure*}

\begin{figure}[h]
    \centering
        \begin{subfigure}{.25\linewidth}
        \centering
        \includegraphics[width=.9\linewidth]{images/taco1.png}
        \caption{}
        \label{subfig:taco1}
    \end{subfigure}%
        \begin{subfigure}{.25\linewidth}
        \centering
        \includegraphics[width=.9\linewidth]{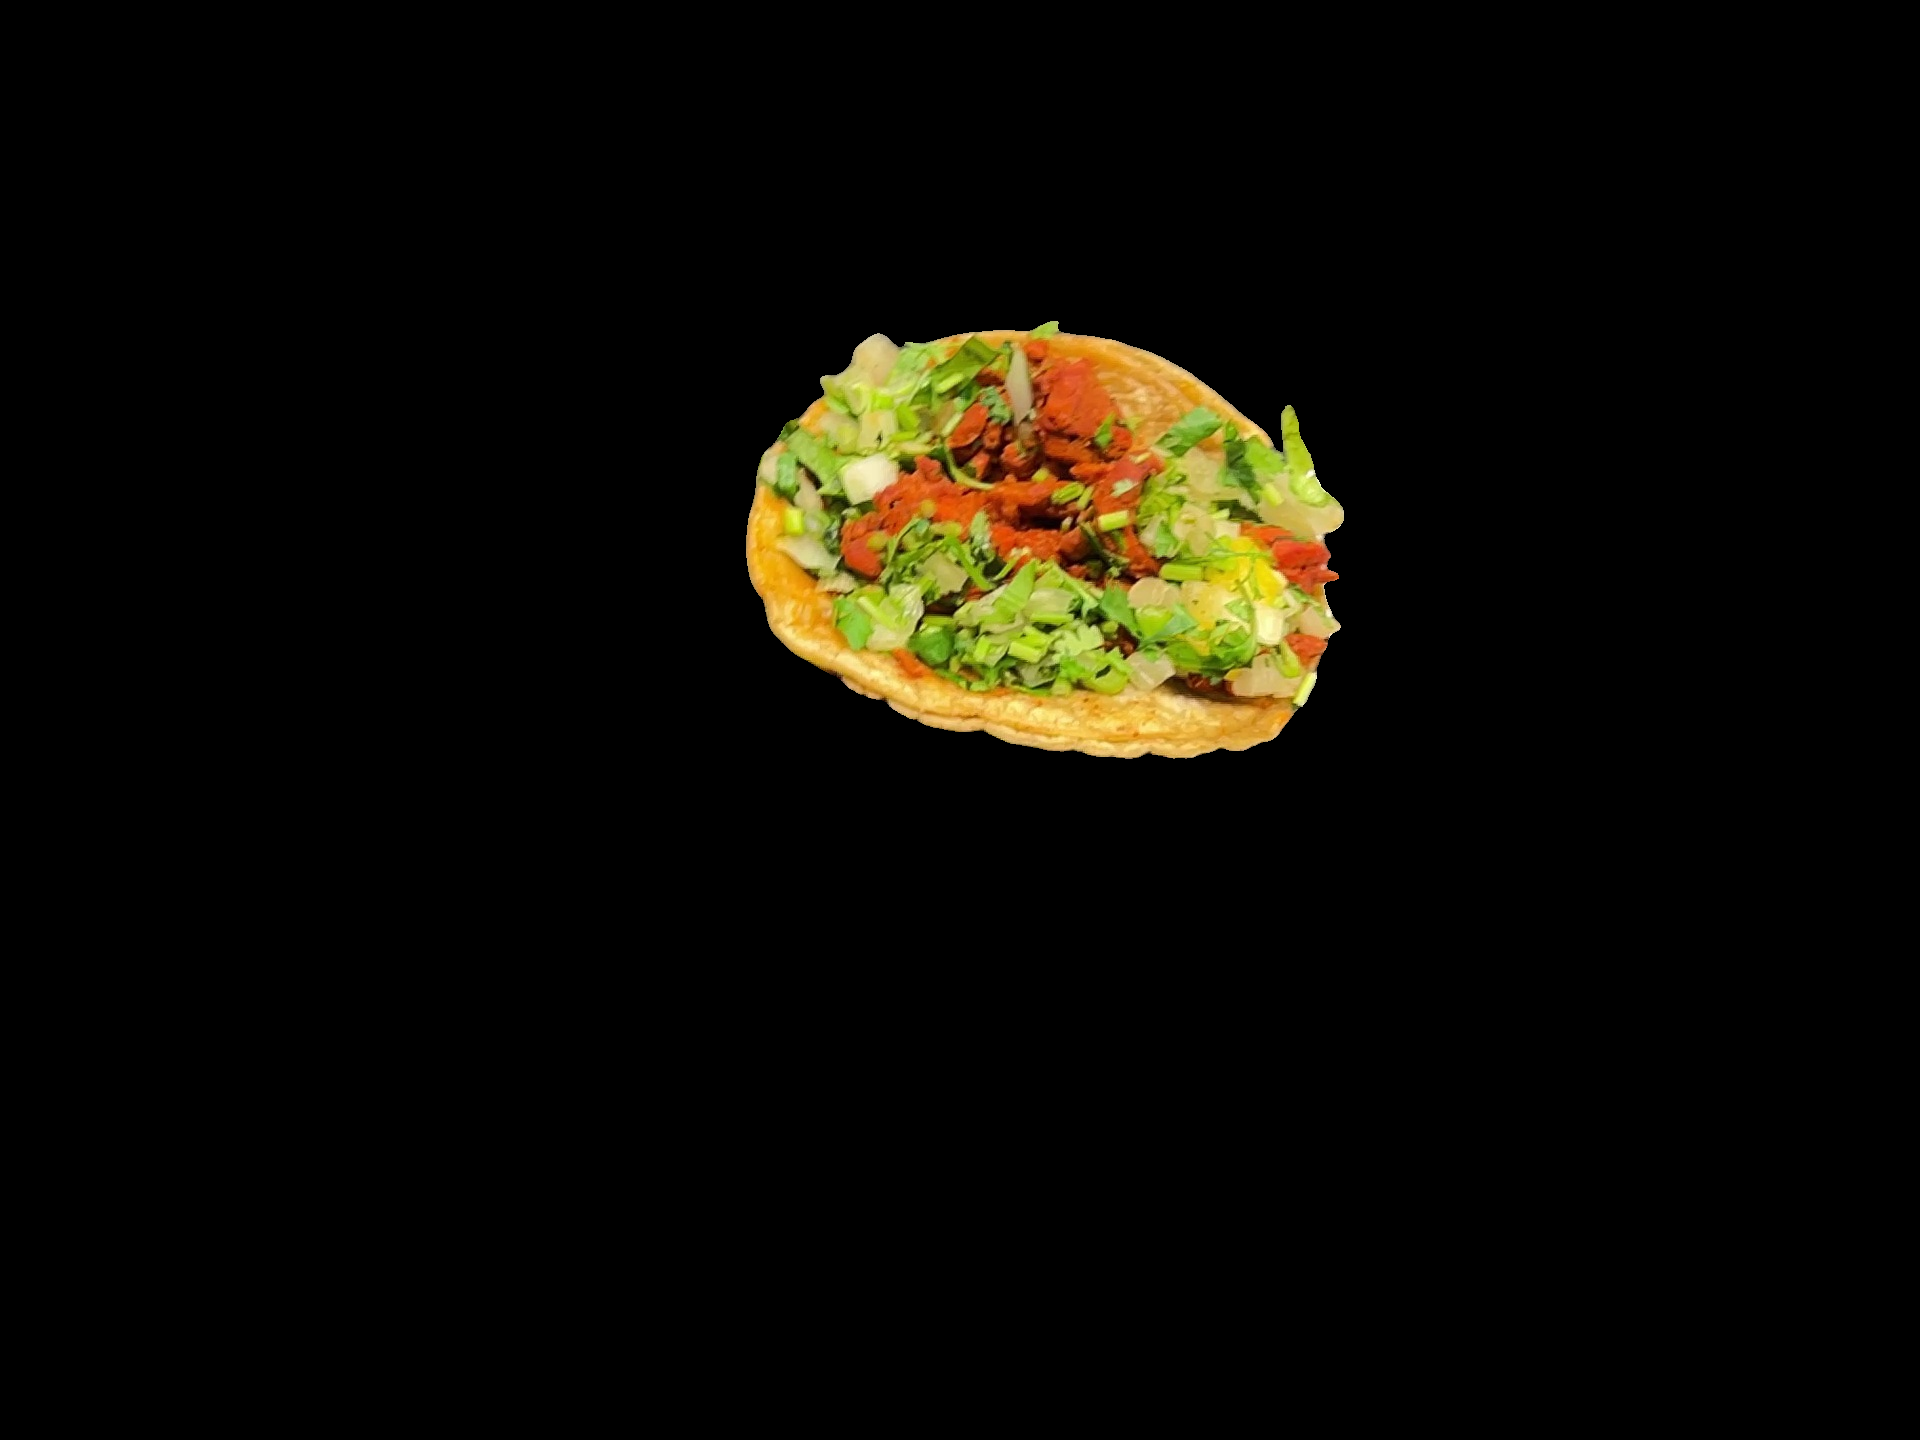}
        \caption{}
        \label{subfig:taco1m}
    \end{subfigure}%
    \begin{subfigure}{.25\linewidth}
        \centering
        \includegraphics[width=.9\linewidth]{images/taco2.png}
        \caption{}
        \label{subfig:taco2}
    \end{subfigure}%
    \begin{subfigure}{.25\linewidth}
        \centering
        \includegraphics[width=.9\linewidth]{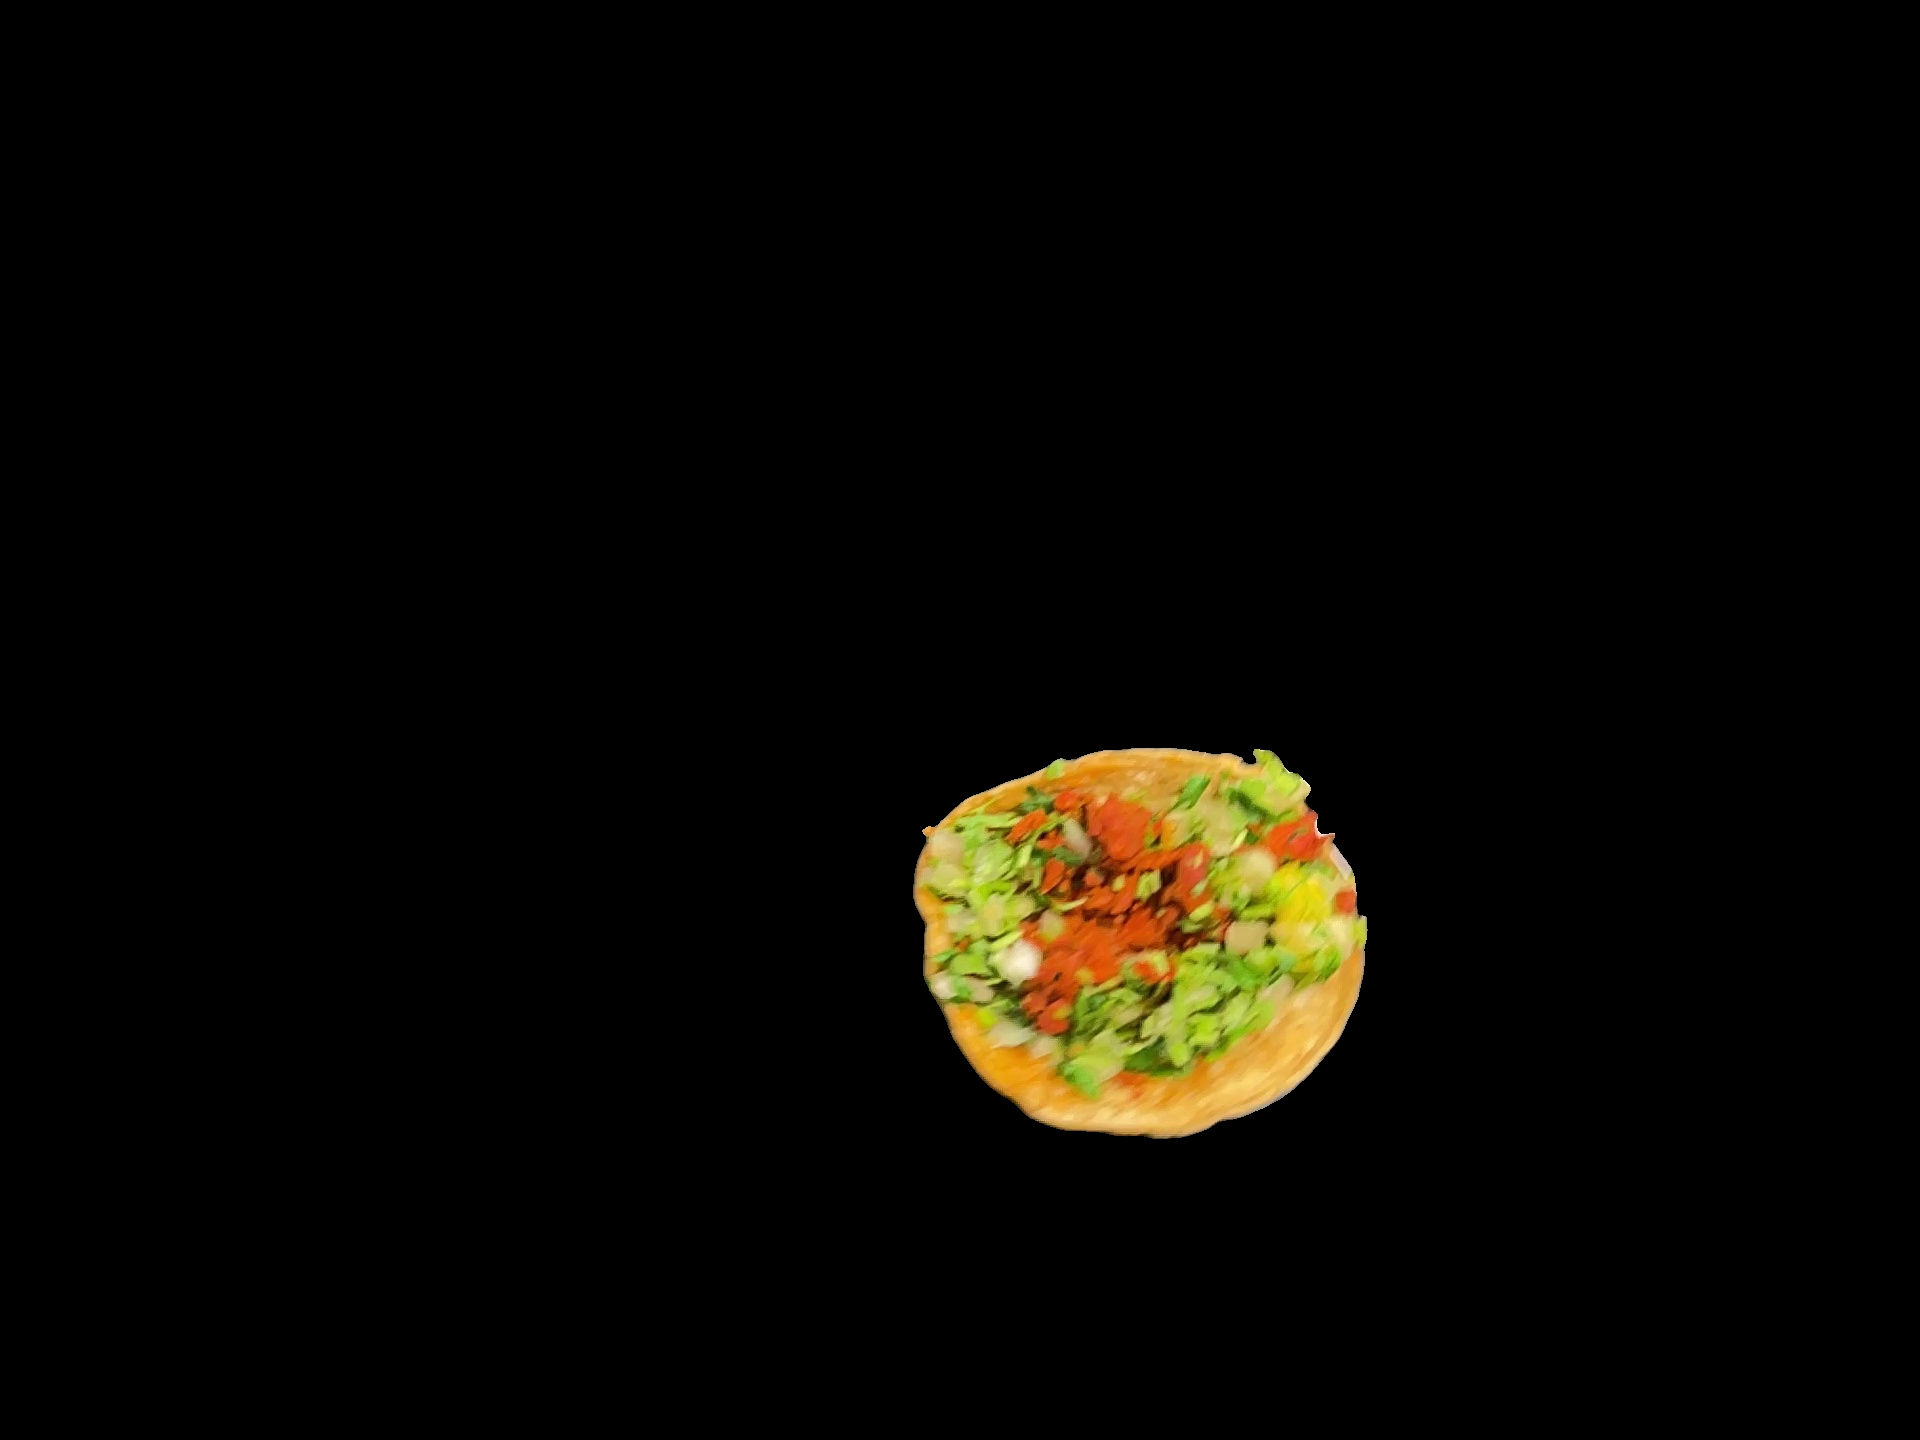}
        \caption{}
        \label{subfig:taco2m}
    \end{subfigure}
    \caption{Example video capture frames with their masks. (a), (c) two example frames for the food object taco, showing different camera views of the same object. (b), (d) results after applying  the provided segmentation masks. }
    \label{fig:video_capture_examples}
\end{figure}

\section{Data Collection Details}
In this section, we provide additional details about our data collection pipeline, illustrated in Figure \ref{pipeline}. Each food object is captured/measured using a scanner, an iPhone app, and a scale. The resulting data are then consolidated and uploaded to our cloud storage. Metadata, along with any potential capture issues, is entered manually. These issues are addressed during the post-processing stage. For RGBD video capture, we employ a 720\textsuperscript{$\circ$} approach by rotating the object twice in a spiral motion, concluding with an overhead capture. Figure \ref{fig:camera_centers} illustrates an example of our video capture camera trajectory computed using COLMAP \cite{schoenberger2016sfm}. As depicted, our camera movements are varied and noisy, effectively reflecting real-world capture scenarios. To ensure precise scale and color measurements of the video capture, we include calibration fiducial markers \cite{xu2012image-FM} in the video, as shown in Figures  \ref{fig:markers}(a) and \ref{fig:markers}(b). The dimensions and colors of the markers are provided in the dataset. Additionally, the POP2 scanner required a dark-colored background for accurate capture. Using a brighter background resulted in parts of the background being erroneously captured by the software as part of the model. Therefore, the turntable and video capture setup were covered with a non-reflective disposable black liner, as shown in Figures \ref{fig:markers}(c) and \ref{fig:markers}(d).

\begin{figure*}[t]
    \begin{center}
        \includegraphics[scale = 0.35]{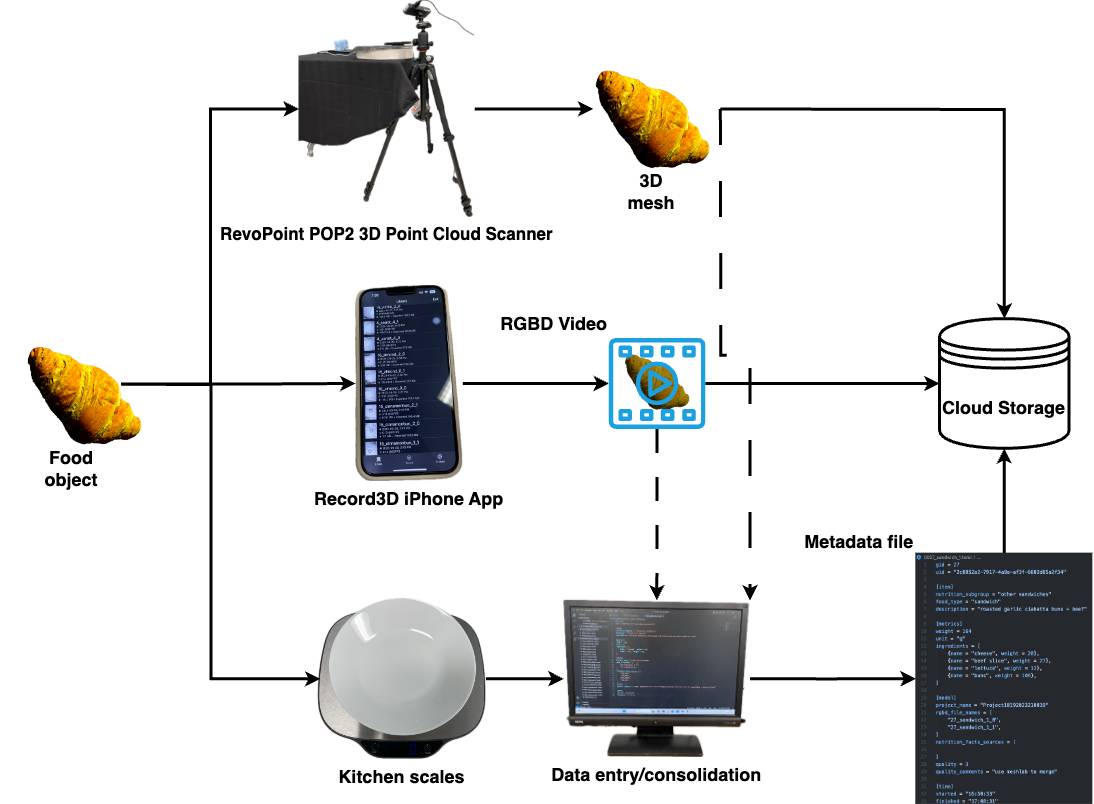}
    \end{center}
    \caption{Data collection pipeline used for the MetaFood3D dataset.}
    \label{pipeline}
\end{figure*}

\begin{figure}
    \centering    \includegraphics[width=\linewidth]{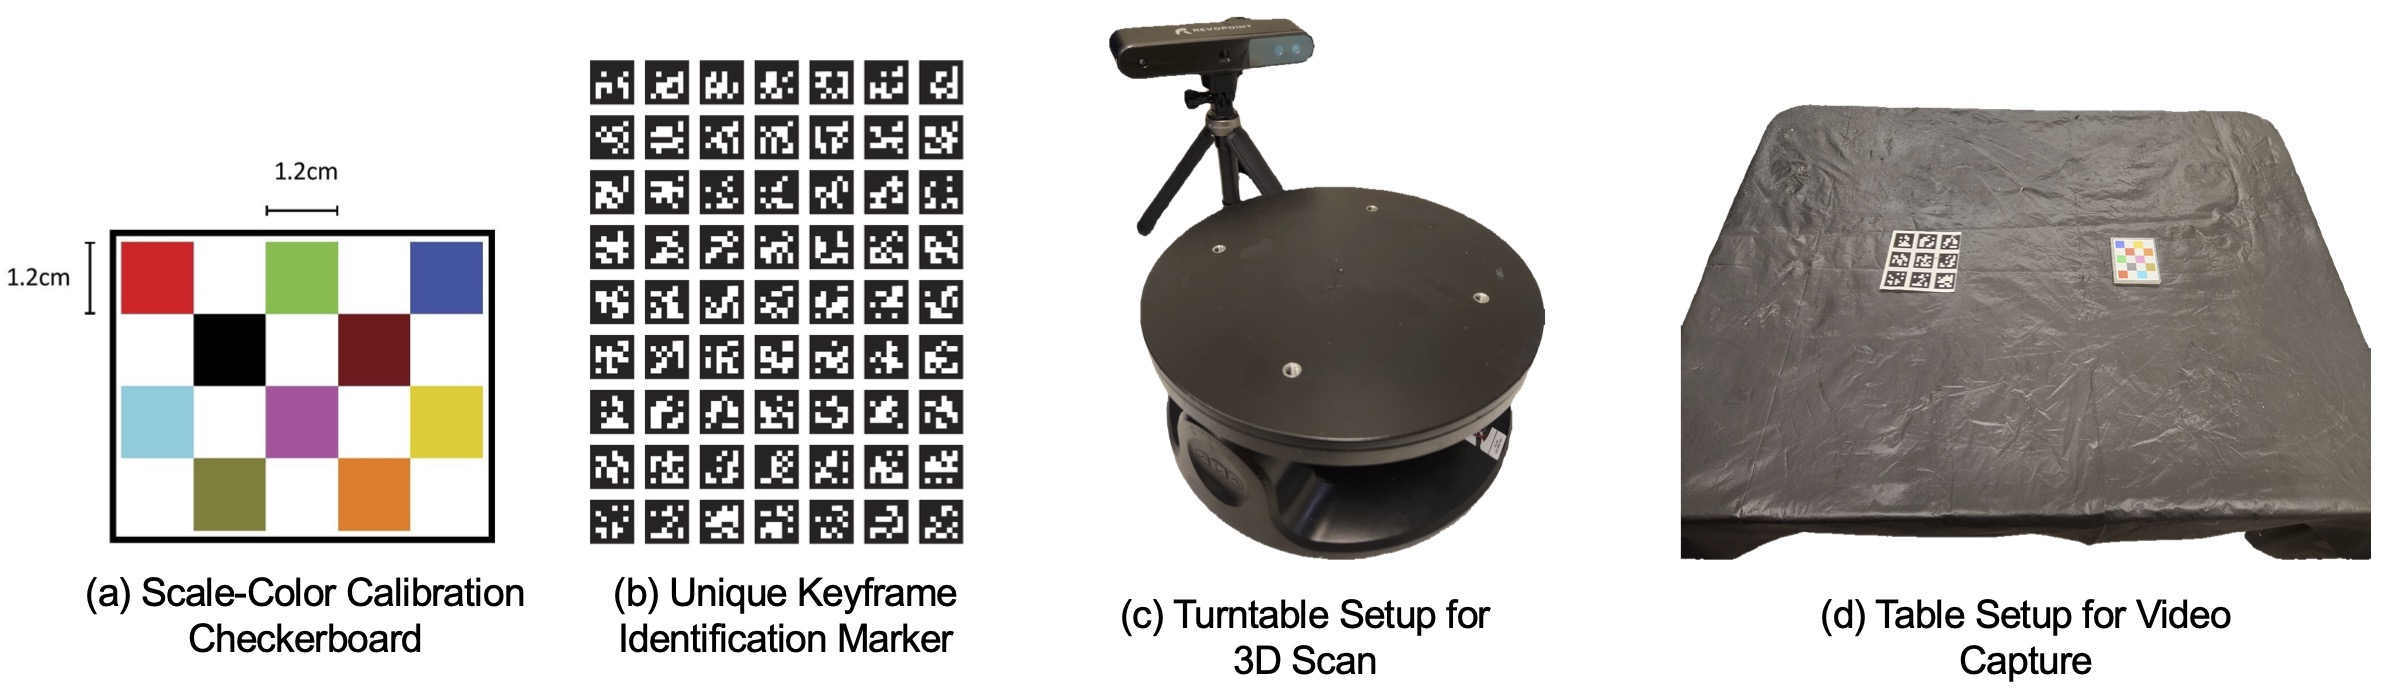}
    \caption{Data capture physical setup elements.}
    \label{fig:markers}
\end{figure}

% \begin{figure}[h]
%     \begin{center}
%         \includegraphics[scale = .2]{images/figure10_new.jpg}
%     \end{center}
%     \caption{Data capture physical setup elements.}
%     \label{fig:markers}
% \end{figure}

\begin{figure}[h]
    \centering
    \begin{subfigure}{.35\linewidth}
        \centering
        \includegraphics[width=.9\linewidth]{images/camera_centers_side_s.png}
        \caption{}
        \label{subfig:centers_side}
    \end{subfigure}%
    \begin{subfigure}{.35\linewidth}
        \centering
        \includegraphics[width=.9\linewidth]{images/camera_centers_top_s.png}
        \caption{}
        \label{subfig:centers_top}
    \end{subfigure}
    \caption{Example camera centers for video capture. Our setup involves a 720-degree capture of the food object from various camera angles, concluding with a top-down view. (a) Side view of the camera trajectory. (b) Top view of the camera trajectory.}
    \label{fig:camera_centers}
\end{figure}

\textbf{Challenges in data collection:} 
Collection food object data is relatively more challenging than collecting rigid object data. We list the challenges in the following.

\textit{Lighting:} We encountered difficulties in capturing intensely red objects, such as strawberries or tomatoes, under cool lighting. In these cases, the automatic object tracking in the RevoScan software would fail to follow the object on the turntable. We resolved this issue by switching to a warmer light source positioned directly above the turntable.

% TODO: single item vs. bowl of items
% TODO: Objects vs. containers
\textit{Food container:} Certain food items imply ambiguitiy in the method of preparation. For example blueberries could both be depicted as singular berries as well as as a container full of berries, the latter being more representative of what is typically visible in a food scene. For this reason some of the objects in our dataset do contain dishes in view and they are annotated accordingly.
Moreover, some of the food items are fluid or liquid in nature and capturing them without a container would not be physically possible.

% TODO: Thin item capture?
%We have not observed significant issues with the capture of 3D meshes of thin items such as nacho chips, unlike \cite{taiNutritionVerse3D3DFood2023}. However, the textures for thin items have proven flat and unremarkable upon inspection. We addressed this issue using Text2Tex \cite{text2tex}, a diffusion-based texture generation method, prompting with the food item name.

% TODO: Sandwich item capture
\textit{Object perspective inconsistencies:} Certain composite food items such as sandwiches have proven exceptionally problematic. Loose elements of the stuffing in a sandwich, for example salad or ham, upon inversion naturally bend in the opposite direction due to gravity. To address this the flexible parts have been edited out in the inverted view of the mesh.

\textit{Object sizes:} Thin and small objects have yielded few problems. It was more problematic to accurately capture large, oblong objects such as bananas. To ensure good texture quality and point-cloud density the scanner should remain relatively close to the object. For oblong objects the distance to the camera must be increased, as the object must stay within the frame for successful capture. This can be in fact addressed by careful positioning of the item on the turntable and using the shortest possible distance to the camera, ensuring the object is fully visible in the frame. Capturing such objects required multiple trials and was more time consuming than an average object capture. 
% For other large oblong objects that were rigid, such as carrots, a modified capture strategy helped. Impaling the object onto a fixture with a nail, placing the fixture on the turntable vertically and simultaneously rotating the scanner vertically resulted in good-quality scans.

\textit{Reflective objects:} We discovered that shiny or reflective objects posed significant challenges during scanning. The device struggled to synchronize points on these objects due to light reflections. Consequently, we were unable to scan items such as cherries in light syrup or popsicles. These objects have been excluded from our dataset.

\textit{Pile-shaped objects:} Some of the food items we captured were largely unstructured piles, such as shredded carrots. For these objects, we had to take extra care to move them undisturbed from the RGBD capture location to the turntable. To facilitate this transfer, we used a small rectangular piece of black liner, and two individuals were tasked with carefully moving the pile.

%\textit{Textures:} For many objects, the textures captured by RevoScan were of insufficient quality. We have addressed this problem by employing the Text2Tex diffusion model \cite{text2tex} which given a 3D mesh and a text prompt generates a new texture for the mesh. A few qualitative samples are presented in \ref{fig:text2tex}.

%Food objects which were naturally dark often had missing parts in the 3D mesh. In this case we resorted to toggling the \emph{Dark Object} scanning mode in RevoPoint RevoScan software. This naturally resulted in parts of the black background being captured.

%% Capturing the underside
%For most food items we would capture also the underside of the object. Two different solutions have been used here. %For models collected by the team at University of Waterloo, we have conducted typically two scans per object, flipping the object upside down wherever possible and we have subsequently merged the two resulting 3D meshes. 

%% Time statistics
\textbf{Data collection time:} We source our food from restaurants, grocery stores, or by preparing it from scratch. Some food items can be purchased together, but due to perishability, we only purchase small batches at a time. On average, it takes about 10 minutes to source each item.
Each food object requires approximately 20 minutes of work by two people for data collection. The average time spent on post-processing each model is about 40 minutes. In total, each food object requires an average of 1.5 hour of person-hours.

\section{Implementation Details of the Experiments}
In this section, we provide implementation details that were omitted from the experiment section of the main paper due to space constraints.

\subsection{3D Food Perception}

In Table \ref{tab:3d perception-2},  we present the robustness analysis of ten 3D point cloud classification models on corrupted point clouds, including DGCNN \cite{wang2019dynamic} as the baseline. The clean point clouds in MetaFood3D are sampled from ground truth mesh files, making them highly accurate representations of the actual physical models' shapes and true dimensions. However, when using point clouds in practical applications, such as 3D reconstructed point clouds from videos, the resulting point clouds often include distorted scaling, coordinate jitters, or changes in the number of points. Therefore, it is crucial to evaluate the performance of point cloud networks under standardized corrupted test sets, as shown in Figure \ref{fig:3d perception_suppl}.

\begin{figure}[ht]
    \centering
    \includegraphics[width=\linewidth]{images/point_clouds_corruption.pdf}
    \caption{MetaFood3D-C Example: This image illustrates the corruptions of a broccoli. Each row represents a different corruption method, with the degree of corruption increasing from left to right.}
    \label{fig:3d perception_suppl}
\end{figure}

MetaFood3D-C test sets are generated with seven types of corruptions: Scale, Rotate, Jitter, Add-G, Add-L, Drop-G, and Drop-L following the standard pipeline in \cite{ren2022benchmarking}. All models were trained on the clean MetaFood3D train dataset. The overall accuracy on the clean MetaFood3D test set is denoted as OA$_{\text{Clean}}$. The calculation for Corruption Error(CE)\ref{perception:eq1} and mCE\ref{perception:eq2} are consistent with those in \cite{ren2022benchmarking}:

\begin{equation}
CE_i = \frac{\sum_{l=1}^5 (1 - OA_{i,l})}{\sum_{l=1}^5 (1 - OA_{i,l}^{\mathrm{DGCNN}})}
\label{perception:eq1}
\end{equation}

\begin{equation}
mCE = \frac{1}{N} \sum_{i=1}^{N} CE_i
\label{perception:eq2}
\end{equation}

We observed that compared to the baseline model DGCNN, many models exhibit strong robustness to the Drop-G corruption method, while most models show poor robustness to the Add-G corruption method. Additionally, we can see that Point-BERT, which employs Bert-style pretraining, performs exceptionally well under the Scale corruption. On average, PointNet++ and GDANet demonstrate the best robustness to point cloud corruption.

\textbf{Training/Testing Settings}: From left to right, for columns 1 and 2 of Table 2 in the main paper, all models are trained on the OmniObject3D\cite{wu2023omniobject3d} training set. OA$_{\text{Uniform}}$ represents the performance of these models evaluated on the OmniObject3D test set. OA$_{\text{Diverse}}$ represents the performance of these models evaluated on the MetaFood3D test set.

For columns 3 and 4 of Table 2 in the main paper and for the full Table \ref{tab:3d perception-2}, all models are trained on the MetaFood3D training set. OA$_{\text{clean}}$ represents the performance of these models evaluated on the MetaFood3D test set. mCE is calculated based on the performance of these models evaluated on MetaFood3D-C, which is generated with the MetaFood3D test set corrupted by different methods and degrees.

OmniObject3D and MetaFood3D do not have official training/test set splits. Therefore, we used a random split with a ratio of 8:2 for training and testing samples from the same category.

\textbf{Compute Resources}: All 3D point cloud perception models were trained on a single NVIDIA A40. Except for PointNet++, all models training were finished in 3 hours, while PointNet++ took approximately 5 hours. The GPU memory usage for all 3D point cloud perception models was within 5000MB. The learning rate, optimizer, and other hyperparameters were set according to the official repositories of each model. Please refer to the "License information for code used" section for details.
\begin{table*}[t]
    \centering
    \scalebox{1.}{

    \begin{tabular}{lc||ccccccc|c}
        \toprule
        \textbf{} & {OA$_{\text{Clean}}$ $\uparrow$} & {Scale}  & {Jitter} & {Drop-G} & {Drop-L} & {Add-G} & {Add-L} & {Rotate} & {mCE} $\downarrow$ \\
        \midrule
        DGCNN \cite{wang2019dynamic} & \cellcolor{mintblue!20}0.725 & 1.000 & 1.000 & 1.000 & 1.000 & 1.000 & 1.000 & 1.000 & \cellcolor{skyblue!40}1.000 \\
        PointNet \cite{qi2017pointnet} & \cellcolor{mintblue!0}0.672 & 1.274 & \underline{0.900} & \cellcolor{lightpurple}0.889 & 1.050 & \cellcolor{lightred}1.762 & 1.219 & 1.374 & \cellcolor{skyblue!0}1.210 \\
        PointNet++ \cite{qi2017pointnet++} & \cellcolor{mintblue!90}\textbf{0.761} & 1.027 & 0.950 & \cellcolor{lightpurple}\textbf{0.732} & \underline{0.895} & \textbf{0.832} & \textbf{0.752} & \cellcolor{lightred}1.197 & \cellcolor{skyblue!90}\textbf{0.912}\\
        SimpleView \cite{goyal2021revisiting} & \cellcolor{mintblue!70}0.747 & \cellcolor{lightpurple}0.917 & 1.011 & 0.924 & 1.011 & 1.021 & \cellcolor{lightred}1.083 & 0.976 & \cellcolor{skyblue!50}0.992 \\
        GDANet \cite{xu2021learning} & \cellcolor{mintblue!50}0.740 & \underline{0.908} & 0.951 & 0.946 & \cellcolor{lightred}0.993 & \cellcolor{lightpurple}\underline{0.901} & \underline{0.931} & \textbf{0.913} & \cellcolor{skyblue!80}\underline{0.935} \\
        PAConv \cite{xu2021paconv} & \cellcolor{mintblue!10}0.711 & 1.051 & 1.014 & \cellcolor{lightpurple}0.971 & 1.013 & \cellcolor{lightred}1.163 & 1.027 & 1.015 & \cellcolor{skyblue!10}1.036 \\
        CurveNet \cite{xiang2021walk} & \cellcolor{mintblue!60}0.745 & 0.989 & \cellcolor{lightpurple}\textbf{0.807} & \underline{0.855} & 1.005 & \cellcolor{lightred}1.160 & 1.028 & \underline{0.919} & \cellcolor{skyblue!60}0.966\\
        RPC \cite{ren2022benchmarking} & \cellcolor{mintblue!40}0.738 & 0.969 & 0.985 & 0.990 & \cellcolor{lightpurple}\textbf{0.860} & 0.940 & 0.941 & \cellcolor{lightred}1.031 & \cellcolor{skyblue!70}0.959\\
        PointMLP \cite{ma2022rethinking} & \cellcolor{mintblue!80}\underline{0.756}& 0.982 & 1.056 & \cellcolor{lightpurple}0.897 & 0.984 & \cellcolor{lightred}1.294 & 1.077 & 0.942 & \cellcolor{skyblue!20}1.033\\
        Point-BERT \cite{yu2022point} & \cellcolor{mintblue!30}0.729 & \cellcolor{lightpurple}\textbf{0.707} & 1.006 & 0.919 & 0.962 & \cellcolor{lightred}1.334 & 1.101 & 1.059 & \cellcolor{skyblue!30}1.013\\
        \bottomrule
    \end{tabular}
    }
    \caption{Robustness Analysis on Corrupted Point Clouds}
    \label{tab:3d perception-2}
\end{table*}

\subsection{Novel View Synthesis}

We used NerfStudio \cite{nerfstudio} for experiments on Nerfacto \cite{nerfstudio} and the Gaussian Splatting \cite{gaussiansplatting} official repository for experiments on  Gaussian Splatting.

\textbf{Datasets}. Throughout, we used train-test split of 9:1. We randomly split the dataset into train set and test set. The split is recorded and used for all the experiments. For video input, we applied COLMAP for extracting the camera parameters and applied the data processing pipeline from NerfStudio to prepare our datasets. For blender input, we used blender-rendered frames as described in the Annotation paragraph in Section 3 and prepared our dataset in the NerfStudio blender data format. 

\textbf{Training details}. All Nerfacto \cite{nerfstudio} and Gaussian Splatting \cite{gaussiansplatting} models were trained for 30,000 iterations before evaluation. For Nerfacto training, we used the default learning rate of $0.0005$ as defined in the NerfStudio official repository. For Gaussian Splatting training, we used the following default values: position lr of $0.00016$, feature lr of $0.0025$, opacity lr of $0.05$, scaling lr of $0.005$, and rotation lr of $0.001$.

\textbf{Compute resource}. We used a pool of NVIDIA RTX 6000 Ada Generation, NVIDIA GeForce RTX 4090, and NVIDIA RTX A6000 GPUs. As training was done frame-by-frame, GPU memory consumption was low and lower-tier GPUs could be used to reproduce our results. Namely, memory consumption was 3367 MiB for Nerfacto unmasked training, 3565 MiB for Nerfacto masked training, and 4295 MiB for Gaussian Splatting.

\subsection{3D Food Generation}
For our experiments, we utilized GET3D~\cite{gao2022get3d} for 3D generation, following the procedures outlined in the official repository.

\textbf{Image rendering}: For 3D generation, we rendered 1,500 images for each subcategory of food models from our dataset using Blender. For example, if the food model "Apple" consists of 5 different kinds of Apple models, we generated 7,500 images for the Apple category. These images were captured from various angles at a resolution of 512 and included camera parameters such as elevation and rotation.

\textbf{Training details}: Each model was trained individually for 3,500 iterations. A gamma value of 3,000 was used to heavily penalize the discriminator, ensuring accurate representation of the food objects, particularly given the smaller number of sub-models per object category. The training process, using 4 GPUs, took 1.5 days to complete 3,500 iterations, achieving a presentable FID score.

\textbf{Evaluation Metrics}:
To evaluate the geometry we use \textbf{Chamfer Distance} (CD) to measure the similarity between two sets of points in 3D space. 
Let $X \in S_g$ denote a generated shape and $Y \in S_r$ a input reference. To compute $CD$, we first randomly sample $N = 2048$ points $X_p \in \mathbb{R}^{N \times 3}$ and $Y_p \in \mathbb{R}^{N \times 3}$ from the surface of the shapes $X$ and $Y$, respectively~\cite{gao2022get3d}. The ${CD}$ can then be computed as:

\begin{equation}
{CD}(X_p, Y_p) = \sum_{\mathbf{x} \in X_p} \min_{\mathbf{y} \in Y_p} \|\mathbf{x} - \mathbf{y}\|_2^2 + \sum_{\mathbf{y} \in Y_p} \min_{\mathbf{x} \in X_p} \|\mathbf{x} - \mathbf{y}\|_2^2.
\end{equation}
To assess the quality of the generated textures and geometry, we use the \textbf{Fréchet Inception Distance} (FID) metric. Following the implementation in GET3D~\cite{gao2022get3d}, we render 50,000 views of the generated shapes for each category using camera poses randomly sampled from a predefined distribution. All images in the test set are encoded using a pretrained Inception v3 model~\cite{inception_v3}, with the output from the last pooling layer used as the final encoding. The FID metric is then calculated as follows:
\begin{equation}
\text{FID}(S_g, S_r) = \|\mu_g - \mu_r\|_2^2 + \text{Tr}[\Sigma_g + \Sigma_r - 2(\Sigma_g \Sigma_r)^{1/2}]
\end{equation}
where $\mu_g$ and $\Sigma_g$ are the mean vector and covariance matrix of the generated image encoding, and $\mu_r$ and $\Sigma_r$ are the mean vector and covariance matrix of the encoding from the input images. $\text{Tr}$ denotes the trace operation.
 
\textbf{Compute resources}: We utilize 4 NVIDIA A40 GPUs for the 3D generation task. Training each food model individually over 3500 iterations takes approximately 1.5 days. During GET3D training, memory consumption was 33,600 MiB per GPU.

\subsection{Rendering}
\textbf{Texture rendering:}
In the main paper, we provided an example of using a texture generation model, Text2Tex \cite{text2tex}, to change the appearance of a food object. In this section, we present additional qualitative samples, as shown in Figure \ref{fig:texture_generation}. 

\textbf{Parameters and Compute resources}: All example samples were generated on an NVIDIA RTX A6000 GPU. The prompt provided consisted of the category name of the object. Text2Tex was run with default parameters: 20 update steps, 50 DDIM generation steps, an update strength of 0.3, a view threshold of 0.1, and 36 viewpoints. Automated post-processing of the texture was also enabled.

\begin{figure}
    \centering
    \includegraphics[width=\linewidth]{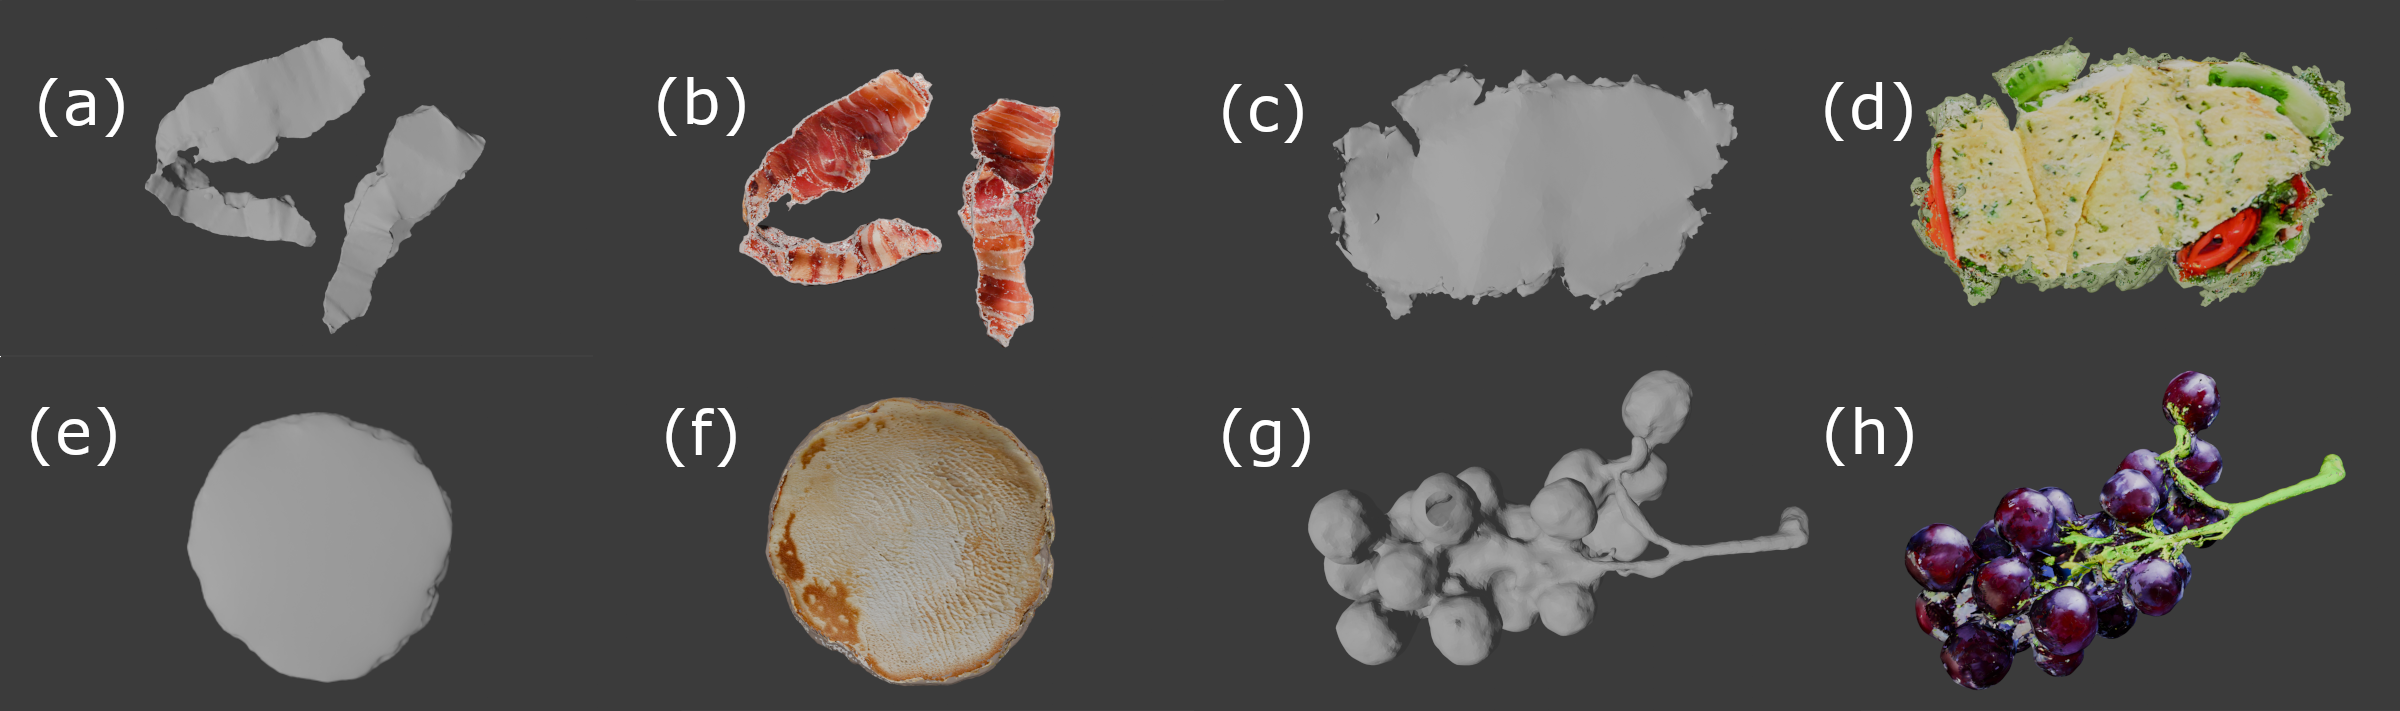}
    \caption{Sample textures generated by Text2Tex. (a, b) Bacon mesh vs. generated texture. (c, d) Omelette mesh vs. generated texture. (e, f) Pancake mesh vs. generated texture. (g, h) Grapes mesh vs. generated texture.}
    \label{fig:texture_generation}
\end{figure}

\subsection{Portion Estimation}
% Table~\ref{tab:portion_estimation} compares different classes of food portion estimation methods.
The metrics used for portion estimation method comparison are:
\begin{equation}
\begin{split}
    \textbf{MAE  } = \frac{1}{N}\sum_{i=1}^N |(\hat{v}_i - v_i)| \\
    \textbf{MAPE (\%)  } = \frac{1}{N}\sum_{i=1}^N \frac{|(\hat{v}_i - v_i)|}{v}
\end{split}
\end{equation}
where $v_i$ is the ground-truth value, $\hat{v}_i$ is the estimated value of the $i$-th image, and $N$ is the number of images in the dataset. 
The main takeaway is the usability of the MetaFood3D dataset for the different input requirements posed by the portion estimation methods. We compare across different classes of methods described in Section~2:

\textbf{Baseline} A model that always predicts the mean value of the field is used. The error between each instance in the dataset and the mean energy or volume of the dataset is established in this baseline. For the Volume MAE (V-MAE) and Volume MAPE (V-MAPE), the mean volume of the dataset is always predicted while for the Energy MAE (E-MAE) and Energy MAPE (E-MAPE) the mean energy of the dataset is always predicted. 

\textbf{Stereo Based Methods} The stereo reconstruction method in \cite{Dehais2017TwoView} describes a process for using 2 images for keypoint detection and matching, stereo rectification, disparity map, and depth map calculation. However, since there is no publicly available implementation, we use the pipeline described in \cite{Dehais2017TwoView} but replace the feature-matching framework with LightGlue~\cite{lindenberger2023lightglue} for better results. The disparity map along with some camera epipolar geometry information is used to project the points to 3D space to obtain a point cloud. The ground-truth segmentation map is used to filter the points to have only the foreground. A scaling factor is obtained for each food type by calculating the mean ratio between the point cloud volume and the ground-truth volume of that food type. Finally, the volume scaling factor of the respective food type is used on the reconstructed point clouds on the test dataset to obtain the volume estimate. 

\textbf{Depth Based Methods} A depth based reconstruction method described in \cite{Fang2016Depth} is implemented with the depth map in the MetaFood3D dataset. The depth map is decoded to actual values using the conversion process detailed by the depth capture mobile app. The RGB image is converted to HSV, the luminosity value scaled from 0 to 3 encodes the depth information in meters. This converted depth map is then used to create a point cloud representation of the scene. The same process applied for the stereo reconstruction is used to scale the point cloud to the actual volume using the point-to-volume ratio of the training dataset. Finally, we obtain the energy from the estimated volume using the same scaling used before.

\textbf{Neural Network Based Methods} Three neural network based methods are implemented, RGB Only (Resnet50)~\cite{Shao2021EnergyDensity}, Density Map Only (ResNet50)~\cite{Vinod2022EnergyDensityDepth} and Density Map Summing~\cite{Ma2023DensityMapSumming}. The neural network based methods are trained to estimate the food energy directly and hence do not have any intermediate volume estimates. In RGB Only (Resnet50)~\cite{Shao2021EnergyDensity} the RGB image serves as an input to a network with a ResNet50~\cite{he2016resnet} backbone feature extractor. The extracted features are then fed to some linear layers with the final linear layer having 1 output which is the estimated energy. The network is supervised on the L1 Loss between the ground-truth energy and estimated energy. For the other methods, we implement the concept of an energy density map. Here, we utilize the ground-truth segmentation maps to understand the area occupied by the foods in the image. Then, the ground-truth energy of the food is distributed uniformly over this area and then scaled to have the pixels maximum value as 255 over the whole dataset. This ``Energy Density Map'' now contains information about the energy of the food. We use the ground-truth energy density map directly via a Resnet50~\cite{he2016resnet} feature extractor, a few linear layers for estimating the energy. Finally, the Density Map Summing~\cite{Ma2023DensityMapSumming} method utilizes this ``Energy Density Map'' and sums up the values of all the pixels and scales it based on the factor used to create the maps. The only error introduced in this approach is the quantization loss resulting from conversion of the ``Energy Density Maps'' to images. For the later couple of methods, the ground-truth ``Energy Density Map'' is used although the original implementation uses a generative model to learn this mapping. However, our implementation should yield better results because the ground-truth maps are used directly. This is done since the ground-truth volume scaling is utilized in the reconstruction methods. Therefore, in order to maintain a fair comparison, the ground truth is utilized directly. Lastly, a 3D point cloud-based network method~\cite{jinge2024MPF3D} was implemented where the 3D point cloud which is reconstructed from the depth map. Since the 3D point-cloud is utilized for portion estimation, the model has a better understanding of the 3D geometry of the food and can thus estimate the volume and energy content of the food with high accuracy.

\textbf{Model Based Methods} The 3D Assisted Portion Estimation~\cite{vinod2024Model3D} utilizes the 3D model of the food to estimate the volume through image rendering and model scaling. For this method, the checkerboard pattern in the image is used to estimate the orientation and translation of the camera and the object in 3D space. Therefore, for the images where the marker was not automatically detected, we manually annotated the corner points as input to the method. Further, only the testing images were used for evaluating the method but the 3D models for each food type were taken from the training dataset. This means that none of the 3D models for any of the images in the testing dataset were used for evaluation. To keep it fair with the other methods, the ground-truth segmentation maps were used. 

The 3D Assisted Portion Estimation~\cite{vinod2024Model3D} and the MFP3D~\cite{jinge2024MPF3D} both of which utilize the 3D models in the MetaFood3D dataset outperform existing methods underscoring the importance of 3D models for food portion estimation and its significant role in the field of nutritional analysis of food.
